# Supplementary material for: Tuning Magnetic Coupling in Sr$_2$IrO$_4$ Thin Films with Epitaxial Strain
Source: arXiv:1312.4005 ancillary file (2014-04-18)
Supplement: Supplementary file 1 [file supplemental_mat_arxiv.pdf]

# Supplemental Material: Tuning Magnetic Coupling in $Sr_2IrO_4$ Thin Films with Epitaxial Strain

A. Lupascu,[1] J. P. Clancy,[1] H. Gretarsson,[1] Zixin Nie,[1] J. Nichols,[2] J. Terzic,[2] G. Cao,[2] S. S. A. Seo,[2] Z. Islam,[3] M. H. Upton,[3] Jungho Kim,[3] D. Casa,[3] T. Gog,[3] A. H. Said,[3] Vamshi M. Katukuri,[4] H. Stoll,[5] L. Hozoi,[4] J. van den Brink,[4] and Young-June Kim[1,*]

[1]*Department of Physics, University of Toronto, 60 St. George St., Toronto, Ontario, M5S 1A7, Canada*
[2]*Department of Physics and Astronomy, University of Kentucky, Lexington, Kentucky 40506, USA*
[3]*Advanced Photon Source, Argonne National Laboratory, Argonne, Illinois 60439, USA*
[4]*Institute for Theoretical Solid State Physics, IFW Dresden, Helmholtzstrasse 20, 01069 Dresden, Germany*
[5]*Institute for Theoretical Chemistry, Universität Stuttgart, Pfaffenwaldring 55, D-70569 Stuttgart, Germany*

(Dated: April 18, 2014)

## OCTAHEDRAL ROTATIONS AND STRUCTURAL DISORDER

To test whether the somewhat unexpected short correlation lengths of the magnetic peaks along the c-axis are related in anyway to the underlying crystal structure, we have investigated the structure of the films in more detail. Neutron and x-rays structural studies have revealed that due to a rotation of the $IrO_6$ octahedra about the crystallographic c-axis, $Sr_2IrO_4$ (SIO) crystallizes with the $I4_1/acd$ space group. [1, 2] This structural distortion is characterized by (1, 2, odd) type superlattice reflections.

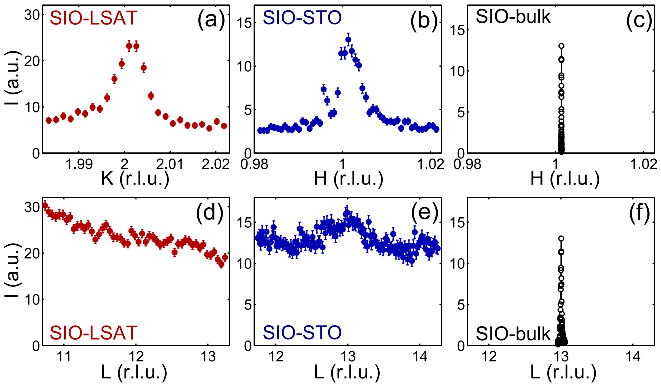


FIG. 1. (a) K-scan and (d) L-scan of the (1 2 13) reflection for SIO-LSAT (red circles) and (b) H-scan and (e) L-scan of the (1 2 13) reflection for SIO-STO (blue circles), at $T = 5$ K. For comparison, the (1 2 13) superlattice peak for SIO bulk (c) K-scan and (f) L-scan, at room temperature, are shown in empty black circles. The H-scan for the bulk is not shown here, but it has a comparable HWHM to the K and L-scans.

Fig. 1 shows scans of the (1, 2, 13) reflection for the SIO-LSAT film along the K-direction (a) and L-direction (b) and for the SIO-STO film along the H-direction (c) and L-direction (d). The scans along the L-direction are extremely broad, or almost flat, for both samples, showing the lack of correlation along the c-axis, in the rotation of the octahedra for these films. The correlation length along the K-direction for the film on the LSAT substrate is $\xi \approx 240 \pm 10$ Å, while the correlation length along the H-direction for the STO substrate is $\xi \approx 300 \pm 10$ Å. These are similar to the magnetic correlation lengths. Just for a rough comparison, we have also included the scans for (1, 2, 17) superlattice peaks of a $Sr_2IrO_4$ single crystal, taken at sector 6-ID at the APS. In contrast to the thin films, the bulk crystal peak is resolution limited along the H, K, and L-direction. Thus, the crystal structure of the thin films could be better described by the I4/mmm space group symmetry, arising from the loss of coherence of the octahedral rotation between the layers. The loss of coherence along the c-direction seems to also be reflected in the magnetic ordering of the films. The magnetic correlation length is *longer* than that of the structure along the c-direction. This could indicate that the magnetic interaction along the c-direction does not depend on the specific superexchange path and perhaps long-range dipole interaction is playing a role.

## ANALYSIS OF THE XRMS MAGNETIC PEAKS

Both thin film samples have the same magnetic ordering wave-vector as the bulk, characterized by the presence of magnetic reflections at (1, 0, L), with L even. To further characterize the magnetic ordering of the $Sr_2IrO_4$ films, we have studied the (0, 1, 14) peak as a function of temperature. The peak profiles, shown in Fig. 2 of the main text were fitted with a Lorentzian function to the n-th power, $I(q) = I_{max}[(q - q_0)^2/(\zeta_n \kappa)^2 + 1]^{-n}$, where $\zeta_n = \sqrt{2^{1/n} - 1}$ is a constant factor set to keep $\kappa$ the half-width at half maximum (HWHM). The parameter $q$ is either H, K, or L, and $q_0$ is the respective peak position. For in-plane scans, n was fixed to 1.5 and a second degree polynomial was used to account for the background contribution. The two adjustable parameters in the fitting function, $I_{max}$ and $\kappa$, are fitted using a nonlinear least-squares fitting procedure. Since the L-scans have a broader profile and a more complex background, the substrate contribution was first subtracted from a

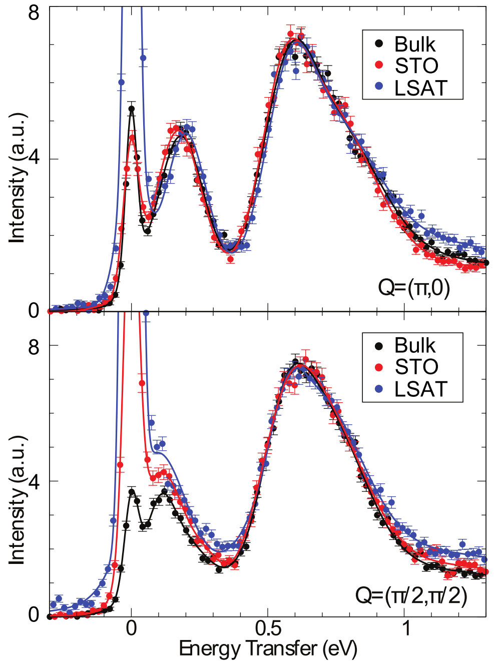


FIG. 2. Effect of epitaxial strain on the characteristic excitations of $Sr_2IrO_4$. A comparison of Ir $L_3$-edge RIXS spectra collected for bulk SIO, SIO-LSAT, and SIO-STO is provided for ($\pi$,0) [upper] and ($\pi/2$,$\pi/2$) [lower] zone boundary wave-vectors. The low-lying excitation (∼100-200 meV) corresponds to the magnon mode discussed in the main text, while the high energy feature (∼600 meV) corresponds to a spin-orbit exciton. The solid lines represent Gaussian fits to the data (collected at room temperature).

high-temperature scan, where the magnetic ordering has already vanished. The background subtracted intensity was also fitted to $I(q)$, with $n = 0.5$ and a constant background. The fitting results are presented in Fig. 3 (a) in the main text.

The observed widths of the film magnetic peaks are approximately 2-3 times broader than the (1,0, 18) bulk magnetic peak along the H and K-direction and an order of magnitude broader than the same magnetic peak along the L-direction, as shown in Fig. 2. In addition, the observed widths of the magnetic peaks are an order of magnitude broader than the instrumental resolution determined from the substrate Bragg peaks ($\approx 0.0005$ r.l.u). We estimated the magnetic correlation length, $\xi$ by inverting $\kappa$: $\xi = \kappa^{-1}$. The epitaxially strained films show similar magnetic correlation lengths, of $\xi \approx 300 - 400$ Å in the ab-plane. The correlation lengths along the c-axis are much smaller: $\xi \approx 10 - 20$ Å (approximately the length of the unit cell).

## ANALYSIS OF THE RIXS SPECTRA

The RIXS spectra provided in Fig. 4 and Supplemental Fig. 2 contain four major features: (1) a strong, sharp, elastic line (E = 0), (2) a dispersive, low-lying magnon mode (E ∼ 100-200 meV), (3) a higher-energy spin-orbit exciton mode (E ∼ 600 meV), and (4) a broad particle-hole continuum (E $\gtrsim$ 400 meV). The spin-orbit exciton mode, in particular, is a unique feature of $Sr_2IrO_4$ which corresponds to onsite transitions between the spin-orbit split levels of the $t_{2g}$ manifold (i.e. the excitation of a hole from the $j_{\rm eff}$=1/2 doublet to the $j_{\rm eff}$=3/2 quartet). In order to extract quantitative information about these features, each spectra was modeled using a multi-Gaussian fit function. A resolution-limited (∼ 45 meV FWHM) Gaussian peak was used to fit the elastic line, while four additional Gaussians were used to describe the magnon (peak 1), the spin-orbit exciton (peaks 2 and 3), and the particle-hole continuum (peak 4). This fitting procedure is similar to the approach which was previously used to model the excitation spectra of bulk $Sr_2IrO_4$ [3].

The RIXS spectra provided in Supplemental Fig. 2 serve to illustrate two significant points. Firstly, we note that the **Q**-dependence of the magnon and spin-orbit exciton modes appear to be qualitatively similar in bulk SIO and the epitaxially-strained thin film samples. The magnons observed in the thin film samples are still strongly dispersive, reaching a maximum energy at the ($\pi$,0) zone boundary position and an energy of approximately half that value at the ($\pi/2$, $\pi/2$) position. The spin-orbiton mode exhibits more subtle dispersion but displays a similar shift in spectral weight in all three samples measured. This indicates that the excitation spectrum of $Sr_2IrO_4$ is largely unaffected by the transition from three-dimensional (bulk SIO) to quasi-two-dimensional (SIO-STO, SIO-LSAT) magnetic order, a result which is consistent with the strong in-plane/out-of-plane anisotropy of the system. Secondly, we note that the spin-orbit exciton mode appears to be much less sensitive to the effect of epitaxial strain than the magnon. The ($\pi$,0) and ($\pi/2$, $\pi/2$) energies of the spin-orbit exciton are almost identical in all three samples (within experimental uncertainty), implying a significantly smaller strain-induced energy shift. This may reflect the fact that the energy scale for the magnon is set by the strength of the magnetic exchange interactions (highly sensitive to bond distance), while the scale for the spin-orbit exciton is primarily set by the strength of the spin-orbit coupling (which is a localized atomic property).

## QUANTUM CHEMISTRY CALCULATIONS

The magnetic spectrum of two corner-sharing $IrO_6$ octahedra was obtained on the basis of embedded-cluster multireference configuration-interaction (MRCI) calculations [4]. To accurately describe the charge distribution at sites in the immediate neighborhood [5, 6], we also included in the actual cluster the closest eight $Ir^{4+}$ and 16 $Sr^{2+}$ ions around the reference $[Ir_2O_{11}]$ fragment. The

TABLE I. Details concerning the structural models used for the quantum chemistry calculations. The splittings among the four low-lying magnetic states are also listed (meV). Due to the antisymmetric anisotropic exchange, $\Psi'_S$ and $\Psi'_1$ are admixtures of $\Psi_S = (\uparrow\downarrow - \downarrow\uparrow)/\sqrt{2}$ and $\Psi_1 = (\uparrow\downarrow + \downarrow\uparrow)/\sqrt{2}$.

| | SIO-STO Model I | SIO-Bulk | SIO-LSAT Model I | SIO-STO Model II | SIO-Bulk | SIO-LSAT Model II |
|---|---|---|---|---|---|---|
| $\measuredangle$ Ir-O$_1$-Ir (°) | 157 | 157 | 157 | 160 | 157 | 155 |
| Ir-Ir (Å) | 3.90 | 3.88 | 3.87 | 3.90 | 3.88 | 3.87 |
| $4\times$ Ir-O$_1$ (Å) | 1.99 | 1.98 | 1.975 | 1.98 | 1.98 | 1.98 |
| $2\times$ Ir-O$_2$ (Å) | 2.05 | 2.06 | 2.07 | 2.05 | 2.06 | 2.07 |
| $\Psi'_S$ | 0.0 | 0.0 | 0.0 | 0.0 | 0.0 | 0.0 |
| $\Psi_3 = (\uparrow\uparrow - \downarrow\downarrow)/\sqrt{2}$ | 49.2 | 55.9 | 59.4 | 55.6 | 55.9 | 54.4 |
| $\Psi_2 = (\uparrow\uparrow + \downarrow\downarrow)/\sqrt{2}$ | 50.0 | 56.9 | 60.5 | 56.6 | 56.9 | 55.2 |
| $\Psi'_1$ | 50.1 | 57.0 | 60.5 | 56.8 | 57.0 | 55.3 |

farther solid-state surroundings were modeled as a large array of point charges fitted to reproduce the crystalline Madelung field in the cluster region.

All calculations were performed with the MOLPRO quantum chemistry software [7]. Energy-consistent relativistic pseudopotentials from the standard MOLPRO library were employed for the two magnetically active Ir ions [8]. The valence orbitals at these reference Ir sites were described by basis sets of quadruple-zeta quality supplemented with two $f$ polarization functions [8] while for the bridging ligand we applied quintuple-zeta valence basis sets and four $d$ polarization functions [9], used in earlier studies on $5d$ oxides [10–12]. The other O's at the two central octahedra were modeled by triple-zeta valence basis sets [9]. For the $Ir^{4+}$ and $Sr^{2+}$ neighbors we employed total-ion effective potentials supplemented with [$2s2p2d$] and [$1s$] valence basis functions, respectively [13, 14].

Multiconfiguration reference wavefunctions were first generated by complete-active-space self-consistent-field (CASSCF) calculations [4]. The active space consists of five electrons and three ($t_{2g}$) orbitals at each of the two central Ir sites. The orbitals were optimized for an average of the lowest nine singlet and the nine triplet states. All these states entered the spin-orbit calculations.

In the MRCI treatment, single and double excitations from the six Ir $t_{2g}$ orbitals and the $2p$ shell of the bridging ligand site are taken into account. Similar strategies of explicitly dealing only with selected groups of localized ligand orbitals were adopted in earlier studies on both $3d$ [15–17] and $5d$ [10–12] compounds, with results in good agreement with the experiment [10, 11, 16, 17]. The MRCI was performed for each spin multiplicity, singlet or triplet, as a nine-root calculation. The subsequent spin-orbit treatment was carried out according to the procedure described in Ref. [18]. Only the four low-lying spin-orbit states are relevant for the analysis of the nearest-neighbor magnetic interactions. The higher-lying spin-orbit states imply an excitation energy of at least 0.6 eV. This gap concerns the $j_{\rm eff}=1/2$ to $j_{\rm eff}=3/2$ transitions [10, 19].

The crystal structure reported by Crawford *et al.* [1] was used for bulk SIO and the lattice parameters of Ref. [20] were used for designing the structural models for the strained films. Relevant data are listed in Table I. As discussed in the main text, the magnetic spectrum computed with Model I does a much better job in capturing the trend observed in the experimental RIXS spectra. In particular, the calculations for this structural model show that compressive strain (SIO-LSAT) causes an increase in $J$, while tensile strain (SIO-STO) causes a decrease. Since the Ir-O-Ir bond angle is the same for these geometries and only the interatomic distances vary, the enhancement/reduction of the nearest-neighbor isotropic exchange obviously arises from having stronger/diminished $5d$-$2p$-$5d$ orbital overlap. The splitting between the singlet and the triplet states for bulk SIO is somewhat larger than in Ref. [10] because the modeling of the adjacent Ir sites is here different. As concerns the calculations for Model II, the actual physics is more subtle since a variable Ir-O-Ir bond angle will additionally significantly affect the Dzyaloshinskii-Moriya couplings [21, 22]. The latter would also influence the splittings among the lowest four spin-orbit states. Work on extracting the effective anisotropic couplings in 214 iridates is still ongoing. All that illustrates how extremely sensitive the magnetic properties of SIO are to local structural details. The *ab initio* results also suggest that the primary strain-induced changes in the films are related to variations in bond length rather than bond angle.

* yjkim@physics.utoronto.ca

[1] M. K. Crawford, M. A. Subramanian, R. L. Harlow, J. A. Fernandez-Baca, Z. R. Wang, and D. C. Johnston, Phys. Rev. B **49**, 9198 (1994).
[2] Q. Huang, J. Soubeyroux, O. Chmaissem, I. Sora, A. Santoro, R. Cava, J. Krajewski, and W. P. Jr., J.

Solid State Chem. **112**, 355 (1994).
[3] J. Kim, D. Casa, M. H. Upton, T. Gog, Y.-J. Kim, J. F. Mitchell, M. van Veenendaal, M. Daghofer, J. van den Brink, G. Khaliullin, and B. J. Kim, Phys. Rev. Lett. **108**, 177003 (2012).
[4] T. Helgaker, P. Jørgensen, and J. Olsen, *Molecular Electronic-Structure Theory* (Wiley, Chichester, 2000).
[5] C. de Graaf, C. Sousa, and R. Broer, J. Mol. Struct. (Theochem) **458**, 53 (1998).
[6] L. Hozoi, L. Siurakshina, P. Fulde, and J. van den Brink, Sci. Rep. **1**, 65 (2011).
[7] H.-J. Werner, P. J. Knowles, G. Knizia, F. R. Manby, and M. Schütz, MOLPRO 2012, see http://www.molpro.net.
[8] D. Figgen, K. A. Peterson, M. Dolg, and H. Stoll, J. Chem. Phys. **130**, 164108 (2009).
[9] T. H. Dunning, J. Chem. Phys. **90**, 1007 (1989).
[10] V. M. Katukuri, H. Stoll, J. van den Brink, and L. Hozoi, Phys. Rev. B **85**, 220402 (2012).
[11] N. A. Bogdanov, V. M. Katukuri, H. Stoll, J. van den Brink, and L. Hozoi, Phys. Rev. B **85**, 235147 (2012).
[12] N. A. Bogdanov, R. Maurice, I. Rousochatzakis, J. van den Brink, and L. Hozoi, Phys. Rev. Lett. **110**, 127206 (2013).
[13] H. Stoll, (2013), (unpublished).
[14] P. Fuentealba, L. von Szentpaly, H. Preuss, and H. Stoll, J. Phys. B **18**, 1287 (1985).
[15] K. Fink, R. Fink, and V. Staemmler, Inorg. Chem. **33**, 6219 (1994).
[16] A. B. van Oosten, R. Broer, and W. C. Nieuwpoort, Chem. Phys. Lett. **257**, 207 (1996); R. Broer, L. Hozoi, and W. C. Nieuwpoort, Mol. Phys. **101**, 233 (2003).
[17] C. J. Calzado, S. Evangelisti, and D. Maynau, J. Phys. Chem. A **107**, 7581 (2003).
[18] A. Berning, M. Schweizer, H.-J. Werner, P. J. Knowles, and P. Palmieri, Mol. Phys. **98**, 1823 (2000).
[19] B. J. Kim, H. Ohsumi, T. Komesu, S. Sakai, T. Morita, H. Takagi, and T. Arima, Science **323**, 1329 (2009).
[20] J. Nichols, J. Terzic, E. G. Bittle, O. B. Korneta, L. E. D. Long, J. W. Brill, G. Cao, and S. S. A. Seo, Appl. Phys. Lett. **102**, 141908 (2013).
[21] B. H. Kim, G. Khaliullin, and B. I. Min, Phys. Rev. Lett. **109**, 167205 (2012).
[22] N. B. Perkins, Y. Sizyuk, and P. Wölfle, Phys. Rev. B **89**, 035143 (2014).
